# Supplementary material for: CenterGrasp: Object-Aware Implicit Representation Learning for Simultaneous Shape Reconstruction and 6-DoF Grasp Estimation
Source: arXiv:2312.08240 source file (2024-04-05)
Supplement: Supplementary file 1 [file 01_Model_Details.tex]

\section{Model and Training Details}

The full model architecture of \ourName is based on CenterSnap \cite{irshad_centersnap_2022} for the encoder and DeepSDF \cite{park_deepsdf_2019} for the decoder. Opposite to the model inference we first train our proposed decoder in an auto-decoder style to learn our latent embedding space (see \cref{subsec:decoder}). The learned embeddings are then used as labels for training the latent code prediction of the encoder. 

\subsection{Shape and Grasps Decoder}
\label{subsec:decoder}
{\noindent \textit{Model Architecture}:} Our decoder network is a deep multi-layer perceptron based on DeepSDF \cite{park_deepsdf_2019}. 
The input to our decoder is a latent code $\latentVariable \in \realNumber^{32}$ and a coordinate in space $\spaceCoordinate \in \realNumber^{3}$. 
The decoder outputs a scalar value $\sdfValue \in \realNumber$ representing the distance to the closest surface as well as a grasp parameterized through a 9D vector raw grasp output $\graspOutput \in \realNumber^{9}$. The vector consists of three sub vectors, an offset for translation part of the grasp $\graspDelta \in \realNumber{3}$ as well as two rotational components $\graspRotation_1, \graspRotation_2 \in \realNumber^{3}$. We build a true, absolute rotation matrix defined in the object frame $\graspRotationFull \in \realNumber^{3 \times 3}$ by applying the Gram-Schmidt procedure on the two rotational components. Thus, the final, full grasp pose is defined through constructing a transformation matrix using both components $\grasp = \transformation \left( \spaceCoordinate + \graspDelta, \graspRotationFull \right) \in SE(3)$ where the matrix is constructed through
\begin{equation}
    \transformation \left( \boldsymbol{t}, \boldsymbol{R} \right) = 
    \begin{bmatrix}
         \boldsymbol{R} &  \boldsymbol{t} \\
        \boldsymbol{0} & 1
    \end{bmatrix}
\end{equation}
where $\boldsymbol{t} \in \realNumber^{3}$ and $\boldsymbol{R} \in \realNumber^{3 \times 3}$.

{\noindent \textit{Labels}:} First, to generate a point-level labeled dataset we use 
\verb|mesh_to_sdf|\footnote{\href{https://github.com/marian42/mesh_to_sdf}{https://github.com/marian42/mesh\_to\_sdf}} 
to sample 300000 points and their respective SDF values. Second, as mentioned in Sec. 3.5 at each point $\spaceCoordinate$ we leverage ACRONYMs \cite{acronym2020} grasping labels by finding the translatory closest successful grasp in ACRONYM. The rotation remains absolute expressed in the object frame.

{\noindent \textit{Training}:} We train the decoder using multiple losses: first, we impose a loss on clamped SDF values 
\begin{equation}
    \lossGeneralFunction_\text{SDF} = 
        \frac
        {            
            \sum_{
                \sdfValue_\text{gt}, \sdfValue_\text{pred} \in \allSdfValues
            }
            \left| 
                \text{clamp} \left( \sdfValue_\text{gt}, \clampThreshold \right)
                -
                \text{clamp} \left( \sdfValue_\text{pred}, \clampThreshold \right) 
            \right|
        }{
            | \allSdfValues |
        }
\end{equation}
where $\allSdfValues$ is the set of all ground truth $\sdfValue_\text{gt}$ and predicted $\sdfValue_\text{pred}$ SDF values. The clamping function 
\begin{equation}
    \text{clamp} \left( x, \clampThreshold \right) = 
        \min ( \max ( x , -\clampThreshold ), \clampThreshold )
\end{equation}
clamps a value $x$ to be between the specified range. In our experiments we used $\clampThreshold=0.1$

Second, we use a 5-point grasp pose loss similar to \cite{sundermeyer2021contact}. We use five  3D points on the gripper defined in the gripper frame, make them homogeneous and stack them, we denote the resulting matrix as $\gripperPoints \in \realNumber^{4 \times 5}$. To accommodate for symmetry we flip the points along the x-y-plane, resulting in $\gripperPointsFlipped \in \realNumber^{4 \times 5}$. We then calculate the grasping loss at each point 
\begin{equation}
    \lossGeneralFunction_\text{Grasp} = \frac
    {
        \sum_{\grasp_\text{gt}, \grasp_\text{pred} \in \allGrasps} \min 
        \left(
            \| \grasp_\text{gt} \gripperPoints - \grasp_\text{pred} \gripperPoints \|,
            \| \grasp_\text{gt} \gripperPointsFlipped - \grasp_\text{pred} \gripperPoints \|
        \right)
    }{
        n_{g}
    }
\end{equation}
where we multiply the ground truth $\grasp_\text{gt}$ and predicted $\grasp_\text{pred}$ grasp with original and flipped gripper point matrix $\gripperPoints$ and use the minimal distance between either of them. The result is averaged over the number of grasps in the batch $n_g$.
Third, we regularize the latent codes through a loss
\begin{equation}
    \lossGeneralFunction_\text{Code} = \bar{\allLatentVariables} 
    \begin{cases}
        \epoch / 5 & \text{if } \epoch < 5 \\
        1 & \text{else}
    \end{cases}\min (1, \epoch / 5) 
\end{equation}
on the mean of all codes $\bar{\allLatentVariables}$ depending on the current training epoch $\epoch$.

We calculate our final loss through
\begin{equation}
    \lossGeneralFunction_\text{decoder} = 
        \lossScaling_\text{SDF} \lossGeneralFunction_\text{SDF} +
        \lossScaling_\text{Grasp} \lossGeneralFunction_\text{Grasp} +
        \lossScaling_\text{Code} \lossGeneralFunction_\text{Code}.
\end{equation}
We report the scaling parameters in \cref{tab:hyper_parameters:decoder}.

We train the network for 75 epochs. We apply dropout with probability 0.2 and weight normalization to regularize training. We use the ADAM optimizer \cite{kingma14adam} with default parameters and a learning rate of $1e-3$.

\subsection{Image Encoder}\label{subsec:encoder}

{\noindent \textit{Model Architecture}:} following the CenterSnap~\cite{irshad_centersnap_2022} architecture, we generate a low-resolution feature representation of both the RGB and depth images using a ResNet~\cite{he2016deep} topology. Both representations are then concatenated and fed into a ResNet18-FPN backbone~\cite{kirillov2019panoptic}. Finally, the resulting pyramid of features is used as input to three specialized heads: a heatmap head, a pose head, and a latent code head. All three network heads output a per-pixel prediction. The architecture of the three network heads is taken from the PanopticFPN~\cite{kirillov19panoptic} segmentation head. It takes FPN features as input and merges information from all levels into single output. Each feature level is upsampled to a common dimension and then summed element-wise. Each upsampling stage consists of a 3×3 convolution, group norm [54], ReLU, and 2× bilinear upsampling.
The heatmap head predicts the probability of objectness for each pixel as a scalar value $ o \in [0, 1]$. The code head predicts a 32-dimensional latent vector representing the shape of the object at that pixel and the possible grasp. The pose head predicts the 6D pose of the object at the given pixel as a 12-dimensional vector, which is then reshaped into a 3x4 matrix and projected to a valid homogenous transformation via a procrustes operation \cite{bregier2021deepregression}.

{\noindent \textit{Labels}:} our synthetic data generation pipeline produces for each scene and viewpoint an rgb image, a depth map, an instance segmentation map and pose labels for each object. We generate labels for our heatmap head by fitting gaussian ellipses on each object instance mask. For the pose-map and code-map labels, we use the instance masks to label each pixel of an object with its ground truth pose vector (12-dimensional) and its ground truth code vector (32-dimensional) respectively.

{\noindent \textit{Training}:} our heatmap loss $\lossGeneralFunction_\text{heat}$ is the simple mean squared error between the heatmap labels and the network output. The shape loss $\lossGeneralFunction_\text{shape}$ is calculated as the L1 loss between prediction and ground truth shape-maps, masked by the object masks (because pixels that do not lie on an object, we do not need a prediction). Our pose loss $\lossGeneralFunction_\text{pose}$ is defined for each pixel by our proposed symmetric-aware loss described in Sec. 3.2. The pose loss at each pixel is then weighted by the ground-truth value of the object heatmap, to emphasize higher weight towards the center of the objects, and finally averaged over all pixels. Our final, total loss is the weighted sum of these 3 losses:

\begin{equation}
    \lossGeneralFunction_\text{encoder} = 
        \lossScaling_\text{heat} \lossGeneralFunction_\text{heat} +
        \lossScaling_\text{shape} \lossGeneralFunction_\text{shape} +
        \lossScaling_\text{pose} \lossGeneralFunction_\text{pose}.
\end{equation}

We report the scaling parameters in \cref{tab:hyper_parameters:encoder}.

We train the network for 200 epochs. To improve generalization, we normalize the rgb values to the dataset mean and standard deviation, we augment the depth values with random noise, and we add color jitter augmentation to the rgb images. We use the ADAM optimizer \cite{kingma14adam} with default parameters and a learning rate of $1e-3$.

\include{tables/hyperparameters}
